# Supplementary material for: Leaf water storage and robustness to intermittent drought: A spatially explicit capacitive model for leaf hydraulics
Source: arXiv:2106.08939 ancillary file (2021-06-16)
Supplement: Supplementary file 1 [file supplement.pdf]

# Supplementary Information of *Leaf water storage and robustness to intermittent drought: A spatially explicit capacitive model for leaf hydraulics*

## 1 Supplementary theoretical modeling results of uniform grass leaves with constant parameters

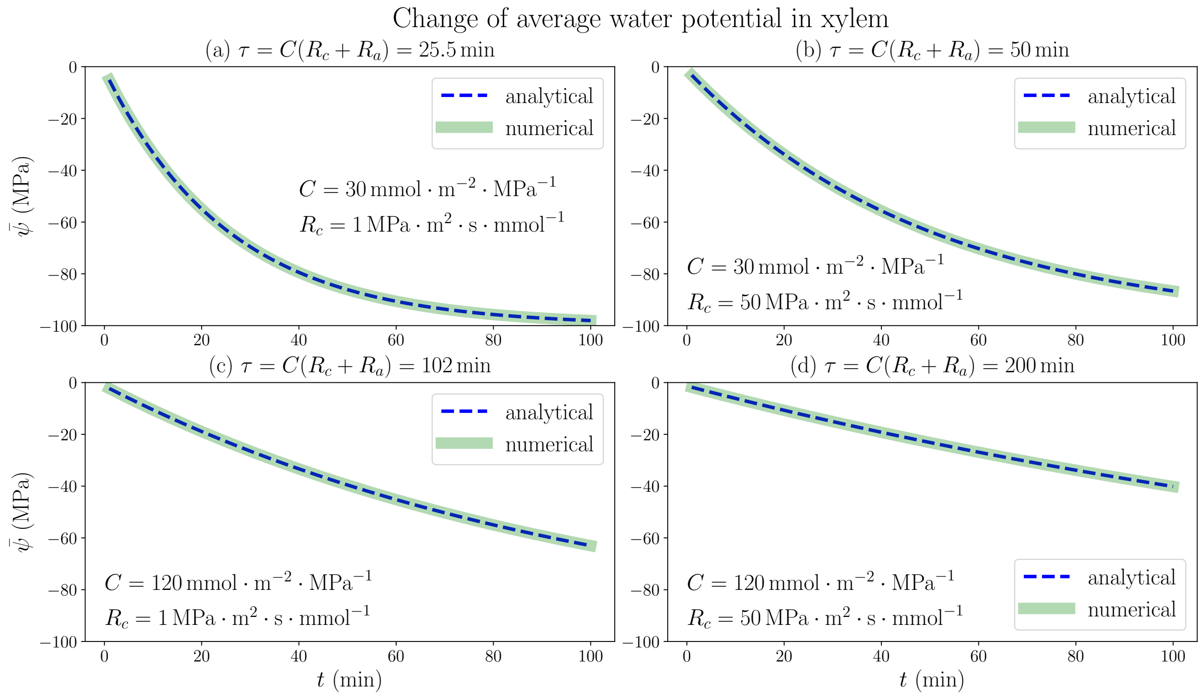


Figure 1: The time dependence of average xylem potential when a living, uniform model leaf in steady state is removed from plant and water source is closed at the base. The 1D simulation results match the analytical exponential decay expressions, with time constants $\tau = C(R_c + R_a)$. The assumption of constant stomatal resistance (and constant $R_a$), which leads to very negative $\bar{\psi}$ in the long term, is highly hypothetical, but is helpful for theoretical investigation. The temporal variations of total transpiration rate are similar. Various sets of whole-leaf capacitance $C$ and xylem-to-capacitor resistance $R_c$ values are used, while other parameters are the same as those in Figure 3 in the main text.

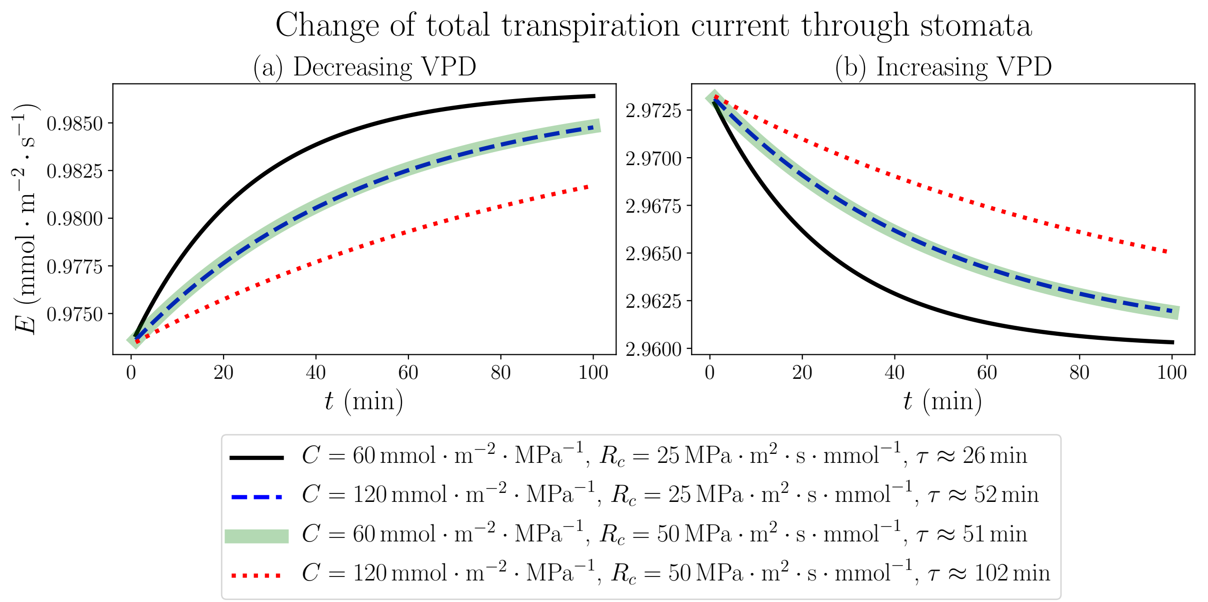


Figure 2: The time dependence of total transpiration rate through stomata, when $\psi_a$ is instantly increased from $-100\,\text{MPa}$ to $-50\,\text{MPa}$ (a, where the air is wetted and VPD is decreased from 1.64 kPa to 0.965 kPa) or decreased from $-100\,\text{MPa}$ to $-150\,\text{MPa}$ (b, where the air is dried and VPD is increased from 1.64 kPa to about 2.1 kPa). Various sets of $C$ and $R_c$ values are used, while other parameters are the same as those in Figure 3 in the main text. In both situations, the time constants $\tau$ corresponding to the same $C$ and $R_c$ values are identical as labeled in the legend. Note that in both (a) and (b) the original transpiration rate at $t < 0$ is $E = 1.97\,\text{mmol}\cdot\text{m}^{-2}\cdot\text{s}^{-1}$, which undergoes an instant change at $t = 0$ and then slightly changes in an exponential way when $t > 0$.

## 2 Experimental measurements of the spatial distribution of water content along *A.villosa* leaf blades

The C4 grass species *Anthaenantia villosa* (*A.villosa*) was used for measuring the local distribution of water amount in its leaves. For light treatment, the species was exposed to light ($\sim 500\,\mu\text{mol}\cdot\text{m}^{-2}\cdot\text{s}^{-1}$) for 1 hour prior to the measurement. For dark treatment, the species was kept in the lab without a light source. Leaf lengths were measured and divided into five segments of equal length marked with sharpies. Sample leaves were cut sequentially from the tip to the base and placed in bags with moist air (except for the dark + 1 hour equilibrium treatment). Leaf fresh mass (FM, g) was measured soon after leaf excision, and leaves were scanned for leaf area (LA, mm$^2$). Segments were dried in a 40 °C oven for > 24 hours for leaf dry mass (DM, g) measurement. For the dark + 1 hour equilibrium treatment, the whole leaf was cut at the base and placed in double bags with moist air for 1 hour in the dark prior to the procedure described above. The purpose of the dark + 1 hour equilibrium treatment was to compare with the dark treatment results to discern any possible statistical difference caused by extra equilibration after excision. Three measurement results were calculated for each segment: leaf mass per unit area (LMA = DM/LA, g/mm$^2$); water amount per unit dry mass (= (FM − DM)/DM, g/g); and water amount per unit leaf area (= (FM − DM)/LA, g/mm$^2$). To account for the effects of both leaf area and thickness on water storage, the water amount per unit dry mass is used to characterize the spatial variations of water content along leaf blades.

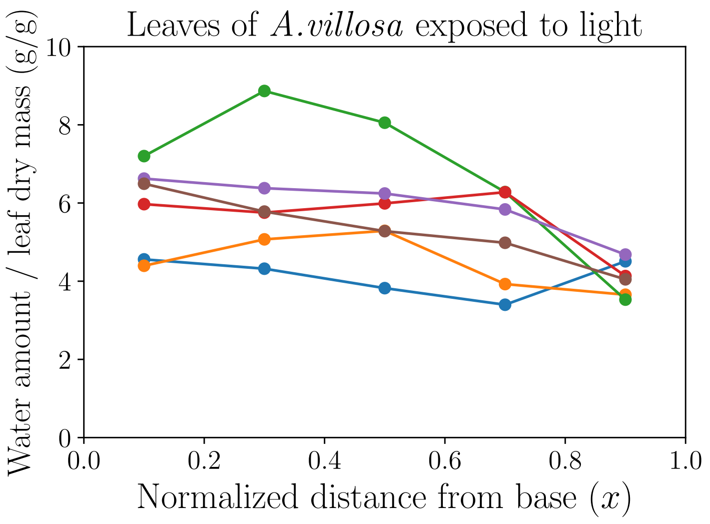


Figure 3: Raw data of local water amount measurements for six *A.villosa* leaves under light treatment.

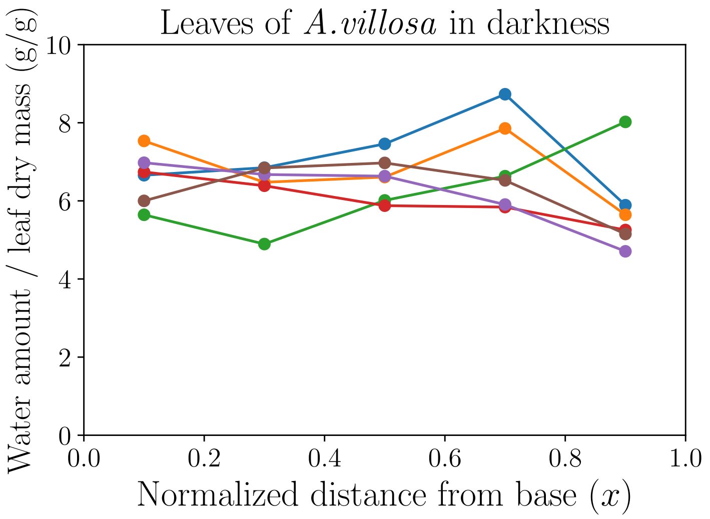


Figure 4: Raw data of local water amount measurements for six *A.villosa* leaves under dark treatment.

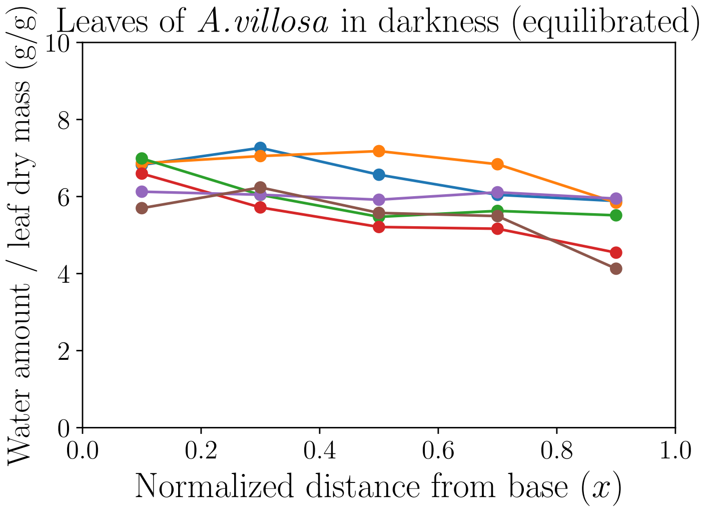


Figure 5: Raw data of local water amount measurements for six *A.villosa* leaves under dark + 1 hour equilibrium treatment.

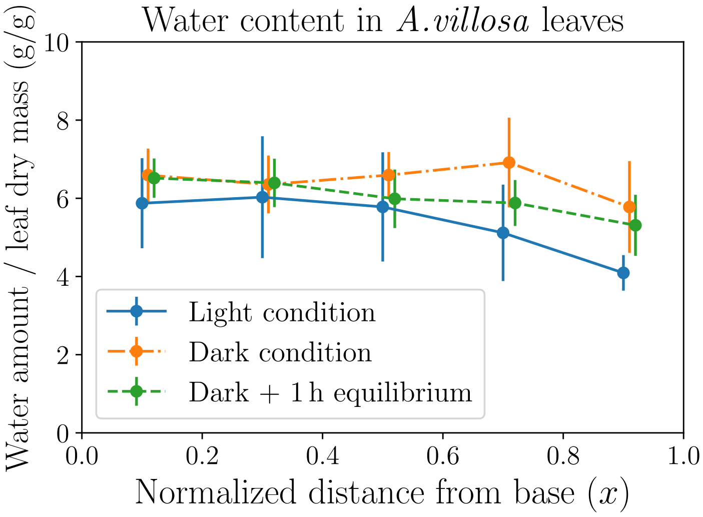


Figure 6: The combined measurement results of *A.villosa* leaves under three different treatments. Error bars represent standard deviations. A more even distribution in leaves in darkness and a tapering trend from base to tip in leaves exposed to light are observed. The leaves equilibrated for an extra hour after excision do not show statistically significant difference from dark treatment results. The three data sets are plotted with a horizontal shift of 0.01 to show error bars.
